# Supplementary material for: Improving Joint Learning of Chest X-Ray and Radiology Report by Word Region Alignment
Source: arXiv:2109.01949 source file (2021-09-04)
Supplement: Supplementary file 1 [file supps.tex]

% This is samplepaper.tex, a sample chapter demonstrating the
% LLNCS macro package for Springer Computer Science proceedings;
% Version 2.20 of 2017/10/04
%
\documentclass[runningheads]{llncs}

%% cross reference setting
\makeatletter
\newcommand*{\addFileDependency}[1]{% argument=file name and extension
  \typeout{(#1)}
  \@addtofilelist{#1}
  \IfFileExists{#1}{}{\typeout{No file #1.}}
}
\makeatother
\newcommand*{\myexternaldocument}[1]{%
    \externaldocument{#1}%
    \addFileDependency{#1.tex}%
    \addFileDependency{#1.aux}%
}
\usepackage{xr}
\myexternaldocument{./paper20}
\usepackage{pbox}
\usepackage[11pt]{moresize}
\usepackage{changepage,threeparttable} % for wide tables
\usepackage{graphicx}
\usepackage{booktabs, multirow} % for borders and merged ranges
\usepackage{soul}% for underlines
\usepackage[table]{xcolor} % for cell colors
\usepackage{amsmath}
\usepackage{amssymb}
\usepackage{makecell}

%% make table/figure labels with "S"
\newcommand{\beginsupplement}{%
        \setcounter{table}{0}
        \renewcommand{\thetable}{S\arabic{table}}%
        \setcounter{figure}{0}
        \renewcommand{\thefigure}{S\arabic{figure}}%
     }
%%

% \myexternaldocument{./2021_MICCAI_joint_image_text}

% \usepackage{booktabs}
% \usepackage{caption} 
% Used for displaying a sample figure. If possible, figure files should
% be included in EPS format.
%
% If you use the hyperref package, please uncomment the following line
% to display URLs in blue roman font according to Springer's eBook style:
% \renewcommand\UrlFont{\color{blue}\rmfamily}

\begin{document}
\title{Improving Joint Learning of Chest X-Ray and Radiology Report by Word Region Alignment} 
% \title{Improving Chest X-Ray and Radiology Report Joint Learning Using Word Region Alignment}
%
\titlerunning{Joint Learning of Chest X-Ray and Radiology Report}
% If the paper title is too long for the running head, you can set
% an abbreviated paper title here
%
\author{Supplemental Material}
\authorrunning{Anonymous}
% First names are abbreviated in the running head.
% If there are more than two authors, 'et al.' is used.

\institute{Anonymous}
% \institute{Princeton University, Princeton NJ 08544, USA \and
% Springer Heidelberg, Tiergartenstr. 17, 69121 Heidelberg, Germany
% \email{lncs@springer.com}\\
% \url{http://www.springer.com/gp/computer-science/lncs} \and
% ABC Institute, Rupert-Karls-University Heidelberg, Heidelberg, Germany\\
% \email{\{abc,lncs\}@uni-heidelberg.de}}
%
\maketitle              % typeset the header of the contrion
%
% \begin{abstract}
% Self-supervised learning provides an opportunity to explore unlabeled Chest X-rays and their associated free-text reports accumulated in clinical routine without manual supervision. This paper proposes a Joint Image Text Representation Learning Network (JoimterNet) for pre-training on chest X-rays and their radiology reports. The model was pre-trained on both the global image-sentence level and the local image region-word level for visual-textual matching, which are both bidirectionally constrained on Cross-Entropy based and ranking-based Triplet Matching Losses. The region-word matching is calculated using the attention mechanism without explicit guidance about their mapping. The pre-trained multi-modal representation learning paves the way for downstream tasks concerning image and/or text encoding. We demonstrate the representation learning quality by multi-label image classifications on two datasets: OpenI-IU and MIMIC-CXR. The fine-tuned encoder initialized with pre-trained representation achieves better classification performance within a shorter training time compared to supervised multi-label classification. 

% \keywords{Self-supervised Learning  \and Multi-modality \and Attention Mechanism.}
% \end{abstract}
%
%
%
\section{Supplemental Materials}
\beginsupplement
% \subsubsection{Hyper-parameter Selection} We first tune the $\gamma$ values in Eq. \ref{eq:prob_sent}, \ref{eq:context_aware_vector}, and \ref{eq:attention_similarity} in order to get the best performing configuration only on $L_{CEM}$ for OpenI-IU dataset. From Table \ref{tab: hyperparameter}(a) the best setting  $\gamma_1,\gamma_2,\gamma_3=1,1,2$ is used while experimenting to find the best margin pair $\eta_w$ and $\eta_s$ for computing TM loss. The best margin setting of $\eta_s, \eta_w=0.5,0.5$ displayed in Table \ref{tab: hyperparameter}(b) is then used to find the best $\lambda$ pair to combine $L_{CEM}$ and $L_{TM}$ shown in Eq. \ref{eq:final_loss}. Finally, the experiment with  $\lambda_{CEM},\lambda_{TM}=4.0, 2.0$ shown in bold in Table \ref{tab: hyperparameter}(c) is used to compute the total loss and achieves the best R@10 of $30.33$ for Image-to-Text and $31.67$ for Text-to-Image retrievals.

\begin{table}[!htp]\centering
\caption{Hyper-parameter selection on a small subset of MIMIC-CXR training set. Experiments in (a) shows the variations in $\gamma$ values for choosing the optimal combination, here $\gamma3$ is same a $\gamma$ in Eq.\eqref{eq:loss_sent}; (b) shows the variations in triplet margin ($\eta$) on the best $\gamma$ combination to choose the optimum margin pair ($\eta_s$, $\eta_w$), here $\eta_w$ is the margin used in region-word-level TM loss $L_{TM}^w$; (c) shows the variations in scaling factor $\lambda$ for choosing the best pair ($\lambda_{TM}, \lambda_{CEM}$) for combining CEM and TM Losses.}
\resizebox{\textwidth}{!}{%
\begin{tabular}{ccc|ccc|ccccccccc|ccc|ccc}
\cline{1-9} \cline{14-21}
\\[-0.9em]
\multicolumn{3}{c|}{} & \multicolumn{3}{c|}{Image-to-Text} & \multicolumn{3}{c}{Text-to-Image} & & & & &
\multicolumn{2}{c|}{} & \multicolumn{3}{c|}{Image-to-Text} & \multicolumn{3}{c}{Text-to-Image} \\
% \cline{4-9} \cline{16-21}
% \\[-1em]
\textbf{$\gamma1$} &\textbf{$\gamma2$} &\textbf{$\gamma3$} &\textbf{R@1} &\textbf{R@5} &\textbf{R@10} &\textbf{R@1} &\textbf{R@5} &\textbf{R@10} & & & & &\textbf{$\eta_{s}$} &\textbf{$\eta_{w}$} &\textbf{R@1} &\textbf{R@5} &\textbf{R@10} &\textbf{R@1} &\textbf{R@5} &\textbf{R@10} \\\cline{1-9}
\cline{14-21}
\\[-1.1em]
100 &10 &10 &1.67 &5.67 &13.67 &1.67 &4.00 &8.33 & & & & &0.5 &1.5 &1.67 &6.00 &18.00 &1.67 &12.67 &24.33 \\
% \\[-1.1em]
10 &5 &10 &4.00 &16.00 &27.33 &2.33 &15.00 &25.67 & & & & &\textbf{0.5} &\textbf{0.5} &\textbf{3.00} &\textbf{16.33} &\textbf{31.33} &\textbf{1.67} &\textbf{18.67} &\textbf{29.33} \\
\cline{14-21}
% \\[-1.1em]
5 &1 &10 &1.33 &5.33 &9.67 &1.33 &5.00 &9.33 & & & & &\multicolumn{8}{c}{(b)} \\
% \\[-1.1em]
4 &5 &10 &1.33 &6.67 &11.33 &0.67 &4.33 &9.33 & & & & &\multicolumn{8}{c}{} \\
% \\[-1.1em]
2 &10 &10 &2.67 &16.67 &27.67 &5.33 &16.00 &24.00 & & & & &\textbf{$\lambda_{TM}$} &\textbf{$\lambda_{CEM}$} &\textbf{R@1} &\textbf{R@5} &\textbf{R@10} &\textbf{R@1} &\textbf{R@5} &\textbf{R@10}\\
\cline{14-21}
\\[-1.1em]
2 &5 &10 &2.00 &11.33 &24.67 &3.33 &14.33 &26.00 & & & & &2.00 &0.75 &3.33 &16.33 &29.00 &4.67 &16.00 &28.00 \\
1 &1 &4 &2.33 &18.33 &28.00 &5.00 &17.00 &27.33 & & & & &1.00 &2.00 &2.67 &12.33 &23.33 &3.67 &12.00 &23.33 \\
\textbf{1} &\textbf{1} &\textbf{2} &\textbf{5.00} &\textbf{17.67} &\textbf{30.00} &\textbf{6.33} &\textbf{18.33} &\textbf{30.33} & & & & &4.00 &1.00 &5.67 &16.00 &28.67 &5.33 &16.33 &25.67 \\
1 &1 &1 &4.00 &11.33 &23.67 &3.00 &12.33 &23.33 & &\textbf{} &\textbf{} &\textbf{} &\textbf{2.00} &\textbf{1.00} &\textbf{5.00} &\textbf{17.67} &\textbf{30.33} &\textbf{6.67} &\textbf{18.67} &\textbf{31.67} \\
\cline{1-9}
\cline{14-21}
% \\[-1.1em]
\multicolumn{9}{c}{(a)} & & & & & \multicolumn{8}{c}{(c)} \\
\end{tabular}}
\\[0.25em]
\label{supptab: hyperparameter}
\end{table}

\begin{table}[!htp]\centering
\caption{Evaluation of negation pattern on manually labelled data points that were originally used for evaluating negation and presented in MIMIC-CXR-JPG paper. Negation was not evaluated for ``NoFinding'' as no cases of negation were labeled. Diseases with less than 5 test samples were considered for evaluation but not displayed in table as the results with such less samples do not convey any information. Note: EC stands for ``Enlarged Cardiomediastinum'', FS stands for training from scratch, FT stands for fine-tuned model. }
\resizebox{\textwidth}{!}{%
\begin{tabular}{l|ccc|ccc|ccc|cccc}\toprule
&\multicolumn{3}{c|}{Precision} &\multicolumn{3}{c|}{Recall} &\multicolumn{3}{c|}{F1-score} &\multicolumn{3}{c}{AUC} \\\cmidrule{2-13}
Negation &NegBio &FS &FT &NegBio &FS &FT &NegBio &FS &FT &NegBio &FS &FT \\\midrule
Cardiomegaly &0.855 &0.860 &\textbf{0.909} &0.720 &0.649 &\textbf{0.722} &0.781 &0.740 &\textbf{0.805} &- &0.918 &\textbf{0.956} \\
Consolidation &0.917 &0.600 &0.704 &0.957 &0.750 &\textbf{0.958} &0.936 &0.667 &0.811 &- &0.985 &\textbf{0.996} \\
Edema &0.713 &0.774 &\textbf{0.852} &0.847 &0.935 &\textbf{0.896} &0.774 &0.847 &\textbf{0.873} &- &0.975 &\textbf{0.975} \\
EC &0.654 &0.500 &0.556 &0.607 &0.333 &0.476 &0.630 &0.400 &0.513 &- &0.782 &\textbf{0.874} \\
Fracture &0.600 &0.500 &\textbf{0.600} &0.375 &0.429 &\textbf{0.429} &0.462 &0.462 &\textbf{0.500} &- &0.513 &\textbf{0.715} \\
Lung Opacity &0.429 &0.500 &\textbf{0.430} &0.391 &0.563 &\textbf{0.500} &0.409 &0.529 &\textbf{0.462} &- &0.816 &\textbf{0.836} \\
Pleural Effusion &0.906 &0.881 &\textbf{0.914} &0.939 &0.912 &\textbf{0.940} &0.922 &0.897 &\textbf{0.927} &- &0.981 &\textbf{0.978} \\
Pneumonia &0.836 &0.825 &\textbf{0.869} &0.735 &0.813 &\textbf{0.828} &0.782 &0.819 &\textbf{0.848} &- &0.966 &\textbf{0.972} \\
Pneumothorax &0.919 &0.920 &\textbf{0.962} &0.955 &0.934 &\textbf{0.961} &0.937 &0.927 &\textbf{0.962} &- &0.979 &\textbf{0.986} \\
\midrule
WeightedAvg &0.831 &0.818 &\textbf{0.865} &0.828 &0.818 &\textbf{0.849} &0.827 &0.814 &\textbf{0.854} &- &0.947 &\textbf{0.963} \\
\bottomrule
\end{tabular}}
\label{supptab: negation}
\end{table}
% No use. Refer to Table \ref{tab: classification_mimic}.

% \textbf{Qualitative Examples} Fig. \ref{fig:qualitative_joimter} illustrates two examples of the region-word alignment attention maps in OpenI-IU dataset. Some critical words such as ``Cardiomediastinal", ``scarring" , and ``atelectasis" have been matched to the reasonable region in the image. 
% \begin{figure}[!htp]
% \begin{center}
% % \fbox{\rule{0pt}{2in} \rule{.9\linewidth}{0pt}}
%   \includegraphics[width=0.6\linewidth]{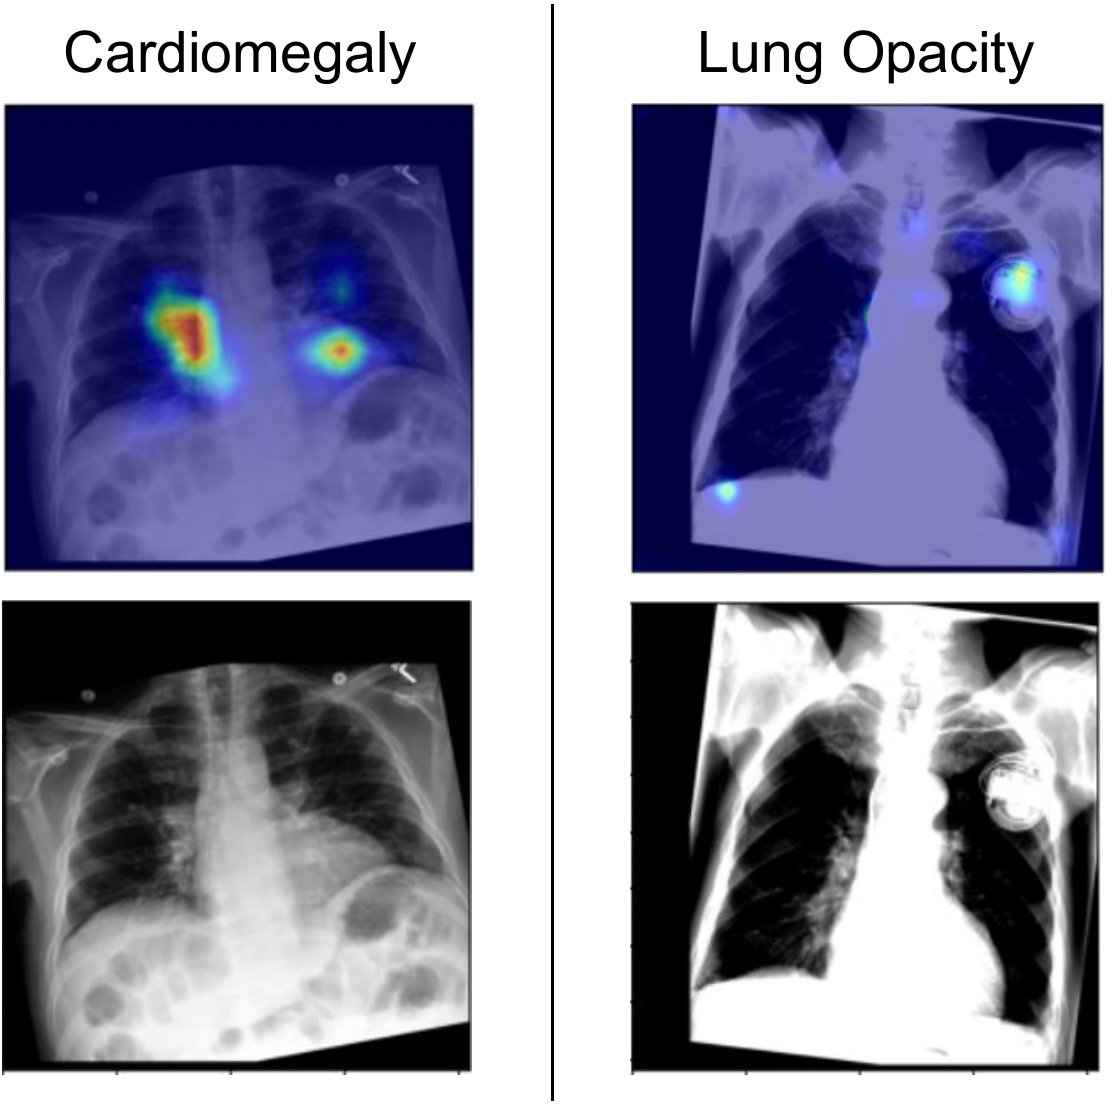}
% \end{center}
%   \caption{Attention maps output from the soft attention layer can automatically identify the location at which the model is focusing.}
% \label{fig:qualitative_joimter}
% \end{figure}

% \begin{figure}[!htp]
% \begin{center}
% % \fbox{\rule{0pt}{2in} \rule{.9\linewidth}{0pt}}
%   \includegraphics[width=1.1\linewidth]{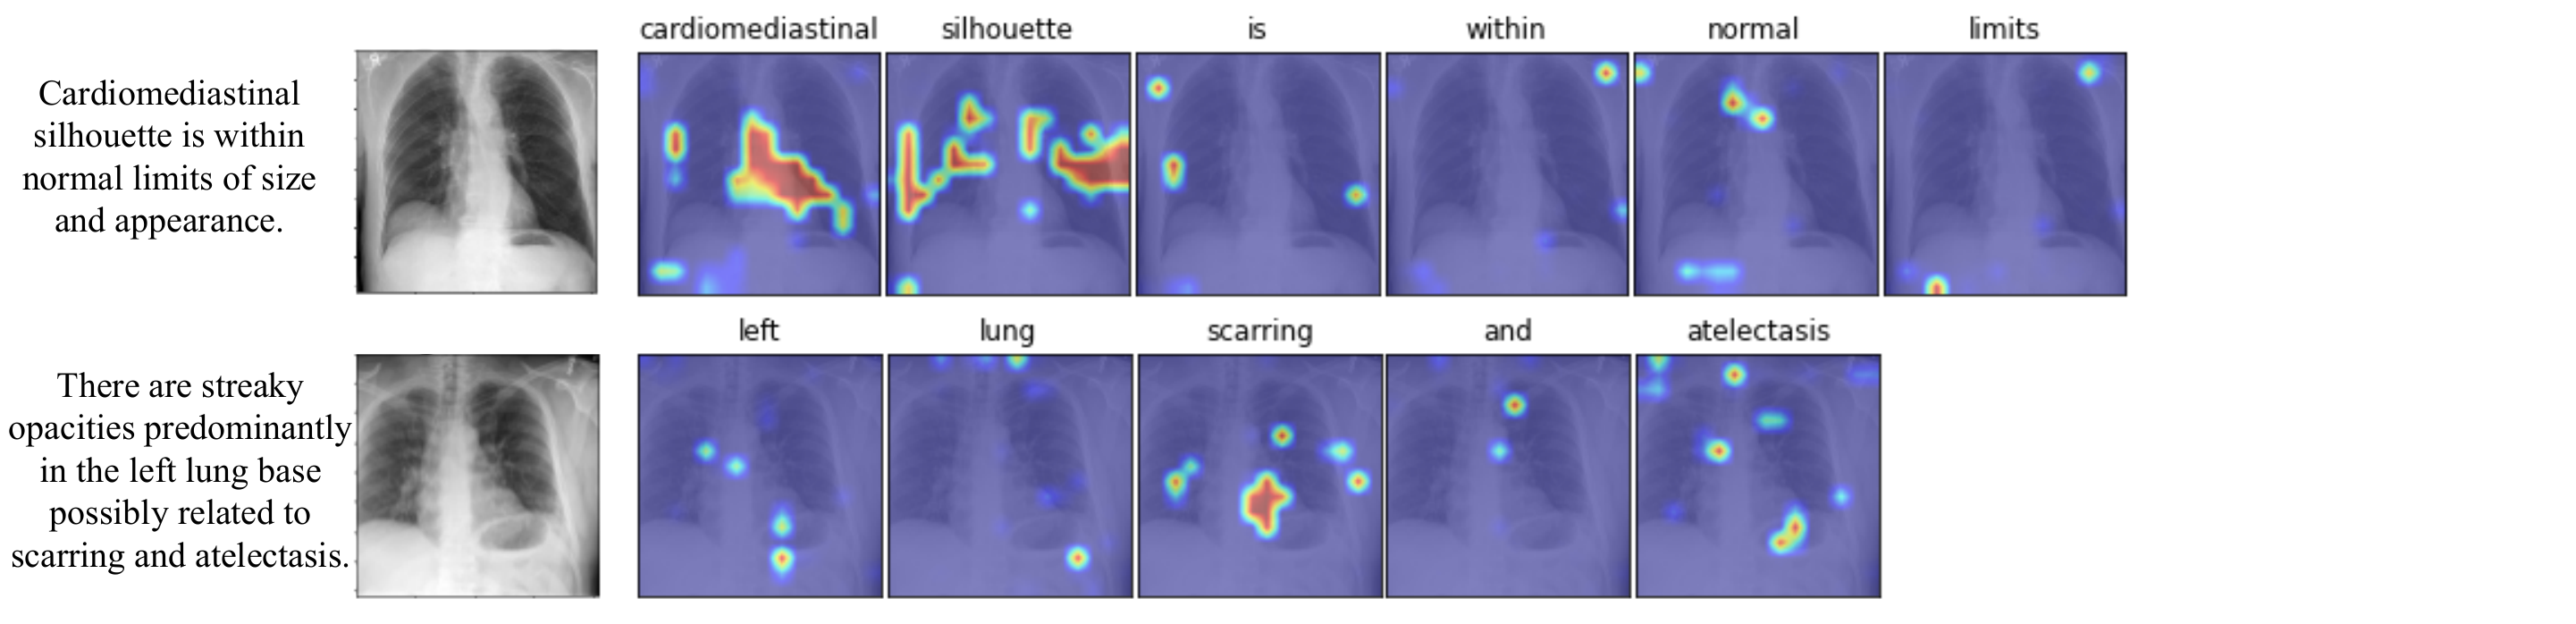}
% \end{center}
%   \caption{The resultant output of word to region alignment attention maps. The first column displays the textual report, the second column displays the radiology image and the rest of the columns show the automatically aligned words and image regions.}
% \label{fig:qualitative_joimter}
% \end{figure}

% \bibliographystyle{splncs04}
% \bibliography{References_MMRL, References_Dana, References_Mingchen}

\end{document}
